# Supplementary material for: Carpe Diem, Seize the Samples Uncertain "At the Moment" for Adaptive Batch Selection
Source: arXiv:1911.08050 source file (2020-12-23)

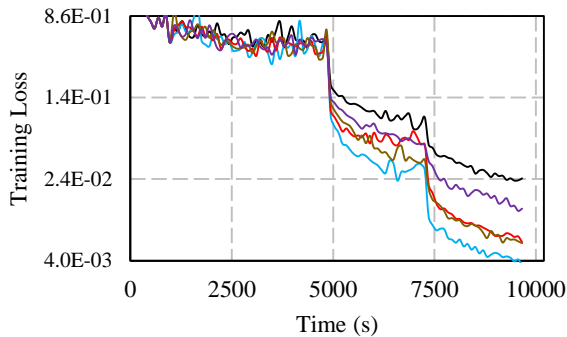

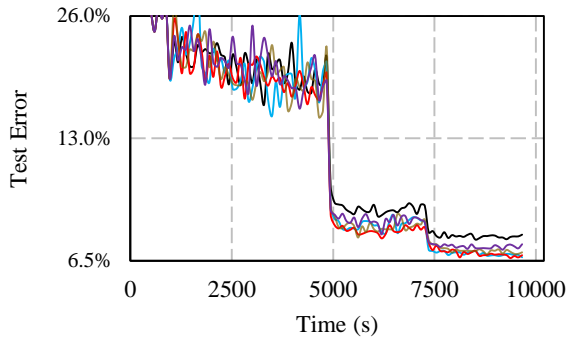

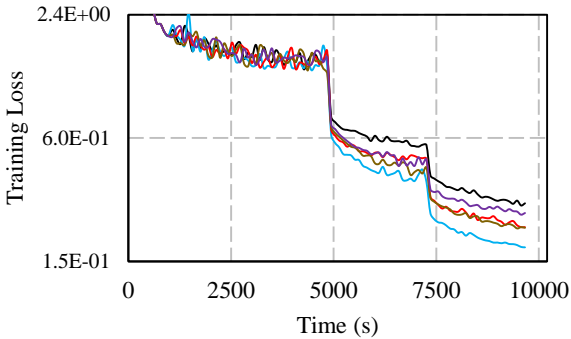

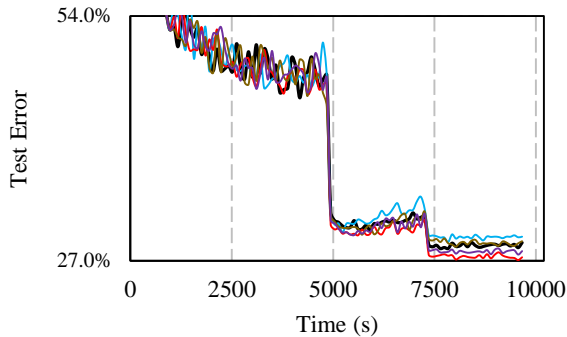

Supplement: Supplementary file 1 [file abalation_densenet.pdf]
